# Supplementary material for: Perspective Flow Aggregation for Data-Limited 6D Object Pose Estimation
Source: arXiv:2203.09836 source file (2022-07-18)
Supplement: Supplementary file 1 [file 6_appendix.tex]

% !TEX root = ../supp.tex
% !TEX spellcheck = en-US

\section{Physical Rendering of SwissCube}
\label{sec:appendix}
